# Supplementary material for: Serving Time: Real-Time, Safe Motion Planning and Control for Manipulation of Unsecured Objects
Source: arXiv:2309.03111 source file (2023-09-06)
Supplement: Supplementary file 1 [file appendix_1.tex]

\section{Newton-Euler Algorithm}
\label{app:nea}

This appendix summarizes the formulas used to recursively compute the angular velocity and acceleration of link $j$ using the angular velocity and acceleration of link $j-1$ and formulas to similarly compute the linear acceleration of each link frame and center of mass of each link.
Note that the angular velocity associated with link $j$ expressed in frame $j-1$ is denoted $\omega\jss$.
Then, the Newton-Euler equations can be used to iteratively calculate the forces and moments both at the CoM of each link and at each joint. 
In particular, we exploit this formulation with the fixed joint between the tray and object in order to calculate the contact wrench.
We use this convention for all quantities of interest not just angular velocities. 
Note for convenience, throughout this appendix, we drop the dependence of the velocity, acceleration, and rotation matrices on the configuration of the robot. 

\begin{lem}[Iterative Newton Euler Formulation] \cite[Ch 6]{Craig2005}
Given the angular velocity of link $j-1$ and the velocity of the robot, one can compute the angular velocity of link $j$ 
    \begin{equation}
        \label{eq:joint_ang_vel}
        \omega\jss = R\jssm \omega\jssmm  + \dot{q}_j \zj.
    \end{equation}
where $\zj$ is the rotation axis vector of the $j^{th}$ joint.
Similarly, given the angular acceleration of link $j-1$, the angular acceleration of link $j$ is:
    \begin{equation}
        \label{eq:joint_ang_accel}
        \begin{split}
        \dot{\omega}\jss = R\jssm \dot{\omega}\jssmm + (R\jssm \omega\jss) \times (\dot{q}_j \zj) + \ddot{q}_j \zj.
        \end{split}
    \end{equation}
The linear acceleration of each link frame is then
    \begin{equation}
        \label{eq:link_lin_accel}
        \dot{v}\jss = (R\jssm \dot{v}\jssmm) + (\dot{\omega}\jss \times p\jssmu) + \left(\omega\jss \times (\omega\jss \times p\jssmu)\right),
    \end{equation}
    and the linear acceleration of the CoM of link $j$ is
    \begin{equation}
        \label{eq:link_COM_lin_accel}
        \dot{v}\jssCOM = \dot{v}\jss + (\dot{\omega}\jss \times p\jssCOM) + \left(\omega\jss \times (\omega\jssa \times p\jssCOM)\right).
    \end{equation}
    Then the inertial force and torque acting at the center of mass of each link is:
    \begin{equation}
        % \label{eq:COM_F_N}
        \label{eq:COM_force}
        F\jss = m_{j} \COMaccel % \GenFGravInert{}
    \end{equation}
    \begin{equation}
        \label{eq:COM_torque}
        \begin{split}
        N\jss = I_{j} \angaccel + \angvel \times \left(I \angvel\right) % \GenMGravInert{}
        \end{split}
    \end{equation}
    where $I_j$ is the spatial inertia matrix of the $j^{th}$ link about it's CoM.
    In addition, the forces and moments acting on the $j^{th}$ link can be defined as: 
    \begin{equation}
        % \label{eq:gen_wrench}
        \label{eq:joint_force}
        \begin{split}
        \genjointforce &= R\jssp f^{j+1}_{j+1} + F\jss,
        \end{split}
    \end{equation}
    \begin{equation}
        \label{eq:joint_torque}
        \begin{split}
        \genjointtorque  = R\jssp n^{j+1}_{j+1}  + c\jss \times \genCOMforce + N\jss 
         + \Big(p\jssp \times \big(R\jssp f^{j+1}_{j+1}\big)\Big)
        \end{split}
    \end{equation}
Then the wrench exerted by the $(j-1)^{th}$ link onto the $j^{th}$ link, through the $j^{th}$ joint, is $\genwrench{j} = \begin{bmatrix} \genjointforce \\  \genjointtorque \end{bmatrix}$.
\end{lem}
When implementing these equations, a Recursive Newton Euler Algorithm (RNEA) is used.
Eqs. \eqref{eq:joint_ang_vel}-\eqref{eq:link_COM_lin_accel} are performed on the forward pass while Eqs. \eqref{eq:joint_force}-\eqref{eq:joint_torque} are performed on the backwards pass, as seen in Alg. \ref{alg:PZRNEA}.
Note that the base case for the backwards pass requires initialization of $f^{\nq+2}_{\nq+2}$, $n^{\nq+2}_{\nq+2}$ and ${R^{\nq}_{\nq+2}}$.
Since we assume no external wrenches are applied to the object, these are initialized to zero vectors for $f^{\nq+2}_{\nq+2}$ and $n^{\nq+2}_{\nq+2}$ and an identity matrix for ${R^{\nq}_{\nq+2}}$.
Further, the effect of gravity on each link is accounted for by initializing the base joint's acceleration to be $a^0_0 = (0, 0, 9.81)^\top \text{m s}^{-2}$ \cite[Sec. 6.5]{Craig2005}.
