# Supplementary material for: Serving Time: Real-Time, Safe Motion Planning and Control for Manipulation of Unsecured Objects
Source: arXiv:2309.03111 source file (2023-09-06)
Supplement: Supplementary file 2 [file appendix_2.tex]

\section{Proof of Lemma \ref{lem:constraint_satisfaction} and Polynomial Zonotope Formulation of the Constraints}
\label{app:slip_proof}

This appendix walks through the formulation of the constraints to prevent $\relativeMotion$ and how they are overapproximated using polynomial zonotopes.
The constraints have to ensure that the object being manipulated does not move relative to the supporting tray.
Therefore, all six degrees of freedom of the object's motion have to be addressed.
In order to form the polynomial zonotope overapproximations, the overapproximation of the contact wrench, $\pz{w_{o}}(\pzqAi, \intparams)$, is used.

\subsection{Vertical Separation Constraint}
    
The first degree of freedom to constrain is translation in the $\hat{z}_{\contact}$ direction, shown in Fig. \ref{fig:contactdiagram}.
Translation \emph{into} the tray is prevented by a reaction normal force from the tray, which is assumed to be a rigid body.
The first constraint on the contract wrench prevents translation \emph{away} from the tray surface.
A violation of this constraint means that the two bodies separate from one another, resulting in no normal force between the two bodies. 
 %Therefore the normal force is equal to the component of the contact force along the z-axis.
Thus this separation constraint can be written as
\begin{equation}
    \label{eq:APPsep_constraint}
    -\czforce(\qA(t;k),\Delta) \leq 0,
\end{equation}
where $\czforce(\qA(t;k),\Delta)$ is the vertical force component of the contact wrench expressed in the contact frame, thus it corresponds to the normal force.
Satisfaction of this constraint means that a normal force exists, and therefore the object is not translating vertically relative to the tray.

The normal component of the contact force is overapproximated by $\pz{f_{\contact,z}}(\pzqAki,\intparams)$, i.e., for each $k\in\pz{K}$ 
\begin{equation}
    f_{\contact,z}(\qA(t;k),\Delta)  \in  \pz{f_{\contact,z}}(\pzqAki,\intparams), \quad \forall t \in \pz{T_i}
\end{equation}
Plugging the overapproximation of the normal force into \eqref{eq:vsep}:

\begin{equation}
    \pz{\sep}(\pz{w^{n_q+1}_{n_q+1}}(\pzqAki, \intparams)) := - \pz{f_{\contact,z}}(\pzqAki,\intparams))
\end{equation}

In order to ensure satisfaction of \eqref{eq:optsepcon}, the polynomial zonotope version of the constraint entails choosing $k$ such that
\begin{equation}
    \label{eq:pz_sepcon}
    % - \pzi{\czforcenotPZ} \leq 0, &\quad  \forall i \in \{1,\hdots,\nt\}
    \setop{sup}(\pz{\sep}(\pz{w^{n_q+1}_{n_q+1}}(\pzqAki, \intparams))) \leq 0, \quad  \forall i \in \{1,\hdots,\nt\}
\end{equation}
Since this constraint is conservatively overapproximative of the actual normal force applied, it is guaranteed that there is a normal force between the loose object and tray when this constraint is satisfied.

\subsection{Linear Slipping Constraint}
    
The next two degrees of freedom, translation in the $\hat{x}_{\contact}$ and $\hat{y}_{\contact}$ directions, can be constrained using a standard Coulomb static friction law. 
The static friction law is formed using the both the normal and tangential components of the contact force. 
Normally, the tangential component would be calculated by taking the norm of the planar contact force components.
However, a square root operation for polynomial zonotopes does not currently exist. 
Therefore, we reformulate the static friction law so that a polynomial zonotope version can be written.
The reformulation is as follows:
\begin{equation}
        \label{eq:static_friction_law}
        |\cforcetan(\qA(t;k),\Delta)| \leq \CoefFric |\czforce(\qA(t;k),\Delta)|
\end{equation}
is equivalent to
\begin{equation}
    \label{eq:static_friction_law_squared}
    \cforcetan((\qA(t;k),\Delta))^{2} \leq  \CoefFric^{2} \czforce((\qA(t;k),\Delta))^{2}
\end{equation}
which can be expanded to 
% \begin{equation}
\begin{align}
    \left(\sqrt{\cxforce((\qA(t;k),\Delta))^{2}+\cyforce((\qA(t;k),\Delta))^{2}}\right)^{2} \\
    \leq \CoefFric^{2} \czforce((\qA(t;k),\Delta))^{2}
\end{align}
% \end{equation}
with the final reformulated slipping constraint written as:
\begin{align}
    \cxforce((\qA(t;k),\Delta))^{2}+\cyforce((\qA(t;k),\Delta))^{2} 
    \\ - \CoefFric^{2} \czforce((\qA(t;k),\Delta))^{2} \leq 0
\end{align}
This constraint requires the tangential components of the contact force to lie within the static friction cone.
Satisfaction of this constraint means that there is no relative linear slip between the object and supporting surface.
% If
% \begin{equation}
%     \label{eq:APPslip_constraint}
%    \slip(\qT(t)) \leq 0,
% \end{equation}
% then the static friction between the object and the tray prevents the object from linearly slipping. 
Note that we do not consider rotational friction for simplicity, but extending the formulation to include such a constraint is a straightforward extension. 

Like the normal component of the contact force, the tangential components are overapproximated by elements of $\pzi{\cwrenchPZ}$.
In particular, for each $k \in K$
\begin{equation}
\begin{split}
    f_{\contact,x}(\qA(t;k),\Delta) \in \pz{f_{\contact,x}}(\pzqAki,\intparams)) \quad \forall t \in \pz{T_i} \\
    f_{\contact,y}(\qA(t;k),\Delta)  \in  \pz{f_{\contact,y}}(\pzqAki,\intparams))  \quad \forall t \in \pz{T_i} 
\end{split}
\end{equation}
The polynomial zonotope terms can be substituted into \eqref{eq:linslip}. 

\begin{align}
    % \begin{split}
         \label{eq:linSlipPZ}
         \pz{\slip}(\pz{w^{n_q+1}_{n_q+1}}&(\pzqAki, \intparams)) := \\
         & \pz{f_{\contact,x}}(\pzqAi,\intparams) \pz{f_{\contact,x}}(\pzqAi,\intparams) \\
         & \oplus \pz{f_{\contact,y}}(\pzqAi,\intparams)\pz{f_{\contact,y}}(\pzqAi,\intparams) \\
         & \ominus \CoefFric^2\pz{f_{\contact,z}}(\pzqAi,\intparams)\pz{f_{\contact,z}}(\pzqAi,\intparams)
    % \end{split}
\end{align}
Then, the polynomial zonotope version of the constraint in \eqref{eq:optslipcon} can be written as
\begin{equation}
    \label{eq:pzslipcon_appendix}
    \setop{sup}(\pz{\slip}(\pz{w^{n_q+1}_{n_q+1}}(\pzqAki, \intparams))) \leq 0
\end{equation}
and by choosing $k$ such that \eqref{eq:pzslipcon_appendix} is satisfied $\forall i \in \{1,\hdots,\nt\}$, it is guaranteed that the object does not translate tangentially to the support surface.

Note that the coefficient of static friction $\CoefFric$ could be uncertain, meaning that the actual coefficient exists in an interval $\CoefFric \in [\mu_{s, lower},\mu_{s, upper}]$.
However, it is only necessary to consider the smallest possible value to ensure no slip occurs, so in \eqref{eq:linSlipPZ}, $\CoefFric=\mu_{s, lower}$, since the static coefficient of friction is always a positive number.
    
\subsection{Tipping Constraint}
    
Finally, we must constrain the last two degrees of freedom, which are rotation about $\hat{x}_{\contact}$ and $\hat{y}_{\contact}$.
Motion about these axes corresponds to the object tipping over. 
To prevent this, we use a Zero Moment Point (ZMP) constraint, which requires that the ZMP point exists inside the convex hull of the contact area of the object \cite{VUKOBRATOVIC2012}.
This ensures that the normal component of the contact force can apply a sufficient counteracting moment to balance the gravito-inertial wrench of the object.
First, let the gravito-inertial wrench acting on the manipulated object be defined as
\begin{equation}
\gravinertwrench{\contact}(\qA(t;k),\Delta) =
\begin{bmatrix}
\FGravInert{}(\qA(t;k),\Delta) \\  \MGravInert{}(\qA(t;k),\Delta)
\end{bmatrix},
\end{equation}
where this wrench, $\gravinertwrench{\contact}(\qA(t;k),\Delta) \in \R^6$, is described in the frame associated with joint $\contact$.
% mention that the wrench is transmitted only through the friction and normal force, which correspond to f_x,f_y,f_z and n_z? so only these components are used to write constraints. 
Next, the vector from $\COMproj{}$ to the ZMP point is \cite[Sec. 2]{VUKOBRATOVIC2012}:
\begin{equation}
    \label{eq:APPZMPpoint}
    \ZMPvec{}(\qA(t;k),\Delta) = \frac{\eenorm{} \times \MGravInertProj{}(\qA(t;k),\Delta)}{\eenorm{} \cdot \FGravInertProj{}(\qA(t;k),\Delta)},
\end{equation}
where 
% $\COMproj{}$ is the point representing the normal projection of the COM of the object onto the supporting surface, $\ZMPpoint{}(\qT(t))$ is the location of the ZMP point, 
$\MGravInertProj{}(\qA(t;k),\Delta)$ is the gravito-inertial moment acting on the object about $\COMproj{}$, and $\FGravInertProj{}(\qA(t;k),\Delta)$ is the gravito-inertial force acting on $\COMproj{}$. 
        % also assuming no other external wrench acting on object so only gravito-inertial wrench needs to be balanced by the supporting surface wrench
        % Need to make sure that the gravito-inertial force and moment are labelled properly. Maybe cite another paper as well? 
        
Next, there are only two wrenches acting on the object, the wrench applied by the manipulator and the gravito-inertial wrench of the object. 
For there to be no relative motion, these two wrenches must balance each other. 
Therefore $\MGravInertProj{}(\qA(t;k),\Delta) = -\cmoment(\qA(t;k),\Delta)$ and $\FGravInertProj{}(\qA(t;k),\Delta) = -\cforce(\qA(t;k),\Delta)$.
Substituting these terms in \eqref{eq:APPZMPpoint} yields
\begin{equation}
    \label{eq:APPZMPpointContact}
    \ZMPvec{}(\qA(t;k),\Delta) = \frac{\eenorm{} \times \cmoment(\qA(t;k),\Delta)}{\eenorm{} \cdot \cforce(\qA(t;k),\Delta)}.
\end{equation}
        % since the negative signs can be factored out and canceled. 
        % \Zac{should probably change the name of $\ZMPvec{}$}
Note that the contact frame is located at $\COMproj{}$, so \eqref{eq:APPZMPpointContact} gives the position of the ZMP point with respect to the origin of the contact frame.
Using the description of the contact patch as in Ass. \ref{assum:contact}, the ZMP constraint can be written as:
\begin{equation}
    \label{eq:rawTipConstraint}
    \left\lVert \frac{\eenorm{} \times \cmoment(\qA(t;k),\Delta)}{(\eenorm{} \cdot \cforce(\qA(t;k),\Delta))} \right\rVert_2 \leq \objrad
\end{equation}
Note that the denominator is a scalar quantity, and so \eqref{eq:rawTipConstraint} can be rewritten as
\begin{equation}
    \left| \frac{1}{(\eenorm{} \cdot \cforce(\qA(t;k),\Delta))} \right| * \lVert \eenorm{} \times \cmoment(\qA(t;k),\Delta) \rVert_2 \leq \objrad
\end{equation}
which is equivalent to
\begin{equation}
    \label{eq:tipConstraintExplained}
    \lVert \eenorm{} \times \cmoment(\qA(t;k),\Delta) \rVert_2 - \objrad \left| \eenorm{} \cdot \cforce(\qA(t;k),\Delta) \right| \leq 0 % \tip(\qT(t)) = 
\end{equation}
If this constraint is satisfied, then the ZMP point stays inside the circular contact area and the object does not rotate about the $\hat{x}_{\contact}$ and $\hat{y}_{\contact}$ axes.

The tipping constraint must also be reformulated to work with polynomial zonotope objects.
The calculation of the tipping constraint, as shown in \eqref{eq:tipConstraint}, requires a square root operation in order to evaluate the $l^2$-norm, which does not currently exist for polynomial zonotopes.
Therefore, we rewrite the constraint as follows:

\begin{equation}
    \lVert \eenorm{} \times \cmoment(\qA(t;k),\Delta) \rVert_2 - \objrad \left| \eenorm{} \cdot \cforce(\qA(t;k),\Delta) \right| \leq 0
\end{equation}
\begin{equation}
    \lVert \eenorm{} \times \cmoment(\qA(t;k),\Delta) \rVert_2 \leq \objrad \left| \eenorm{} \cdot \cforce(\qA(t;k),\Delta) \right|
\end{equation}
\begin{equation}
    \sqrt{(\eenorm{} \times \cmoment(\qA(t;k),\Delta))^2} \leq \objrad \left| \eenorm{} \cdot \cforce(\qA(t;k),\Delta) \right|
\end{equation}
\begin{equation}
    (\eenorm{} \times \cmoment(\qA(t;k),\Delta))^2 \leq \objrad^2 (\eenorm{} \cdot \cforce(\qA(t;k),\Delta))^2
\end{equation}
\begin{equation}
    \label{eq:tipcon_appendix_reform}
    (\eenorm{} \times \cmoment(\qA(t;k),\Delta))^2 - \objrad^2 (\eenorm{} \cdot \cforce(\qA(t;k),\Delta))^2 \leq 0
\end{equation}

Overapproximations of these components are calculated in order to form the polynomial zonotope overapproximation of the tipping constraint.
First, we have that for each $k \in \pz{K}$
\begin{equation}
    \cwrench(\qA(t;k),\Delta) \in \pz{\cwrenchPZ}(\pzqAki,\intparams) \quad \forall t \in \pz{T_i}
\end{equation}
This means that the contact force and moment vector can be overapproximated by the corresponding components of the wrench overapproximation
\begin{equation}
    \begin{split}
        \cmoment(\qA(t;k),\Delta) \in \pz{n_{o}}(\pzqAki,\intparams) \quad \forall t \in \pz{T_i} \\
        \cforce(\qA(t;k),\Delta) \in \pz{f_{o}}(\pzqAki,\intparams) \quad \forall t \in \pz{T_i}
    \end{split}
\end{equation}

The contact force and moment vector overapproximations can be substituted into \eqref{eq:tipcon_appendix_reform}. 
The polynomial zonotope overapproximation of the cross product in \eqref{eq:tipcon_appendix_reform} is
\begin{equation}
    \label{eq:pz_ZMP_numerator}
    \eenorm{} \otimes \pz{n_{o}}(\pzqAi,\intparams) = 
    \begin{bmatrix}
        \pz{d_1}(\pzqAi,\intparams) \\
        \pz{d_2}(\pzqAi,\intparams) \\
        0
    \end{bmatrix}
\end{equation}
and the overapproximation of the dot product in \eqref{eq:tipcon_appendix_reform} is
\begin{equation}
    \label{eq:pz_ZMP_denominator}
    \eenorm{} \odot \pz{f_{o}}(\pzqAi,\intparams) = \pz{d_3}(\pzqAi,\intparams)
\end{equation}
Thus an overapproximation of \eqref{eq:tipConstraint} can be written as
\begin{align}
    \label{eq:pz_tipcon}
    % \begin{split}
    \pz{\tip}(\pz{w^{n_q+1}_{n_q+1}}&(\pzqAki, \intparams)) = \\
    & \pz{d_1}(\pzqAki,\intparams) \pz{d_1}(\pzqAki,\intparams) \\
    & \oplus \pz{d_2}(\pzqAki,\intparams) \pz{d_2}(\pzqAki,\intparams) \\
    & \ominus \pz{d_3}(\pzqAki,\intparams) \pz{d_3}(\pzqAki,\intparams) \objrad^2
    % \end{split}
\end{align}
Then, the polynomial zonotope version of the constraint can be written as 
\begin{equation}
    \label{eq:APPtipConstraint}
    \setop{sup}(\pz{\tip}(\pz{w^{n_q+1}_{n_q+1}}(\pzqAki, \intparams))) \leq 0
    % \begin{split}
    %     \pz{a}(\pzqAi,\intparams) \pz{a}(\pzqAi,\intparams) & \\
    %     \oplus \pz{b}(\pzqAi,\intparams) \pz{b}(\pzqAi,\intparams) & \\
    %     \ominus \pz{d}(\pzqAi,\intparams) \pz{d}(\pzqAi,\intparams) \objrad^2 & \leq 0
    % \end{split}
\end{equation}
By choosing k such that \eqref{eq:APPtipConstraint} is satisfied $\forall i \in \{1, . . . , n_t \}$, it is guaranteed that the object will not tip over.
Similar to the coefficient of friction, the radius of the contact area could be uncertain but only the smallest possible value needs to be considered in order to guarantee that no tipping occurs.
Therefore, in \eqref{eq:pz_tipcon}, if $\objrad \in [\objrad_{lower},\objrad_{upper}]$, then $\objrad = \objrad_{lower}$, since the radius must be a positive quantity.
