# Supplementary material for: Serving Time: Real-Time, Safe Motion Planning and Control for Manipulation of Unsecured Objects
Source: arXiv:2309.03111 source file (2023-09-06)
Supplement: Supplementary file 4 [file appendix_5.tex]

\section{Forward Kinematics and Occupancy Algorithms}
\label{app:pzfkandpzfo}

In this appendix, we present algorithms for calculating the forward kinematics and forward occupancy of an extended manipulator using polynomial zonotopes.

%~~~~~~~~~~~~ Compose FK
\begin{algorithm}[t]
\small
\begin{algorithmic}[1]

% \State{\bf parfor} $i \in \Nt$ %// parallel for each time step

\State{\bf for} $j = 1:\nq+1$ %// for each joint \hspace{0.2in}

    \State\hspace{0.2in} $\pz{p_0}(\pzqi) \leftarrow \zeros$ %// initialize frame location 

    \State$\hspace{0.2in} \pz{R_0}(\pzqi) \leftarrow I_{3 \times 3}$ %// initialize frame orientation
    
    \State\hspace{0.2in}$\pz{R_{j}^{j-1}}(\pzqji), \pz{\nom{p\jssmu}} \leftarrow \pz{\homtrans_{j}^{j-1}}(\pzqji)$ as in \eqref{eq:homogeneous_transform}
    
    \State\hspace{0.2in}$\pz{p_j}(\pzqi) \leftarrow \pz{p_{j-1}}(\pzqi) \oplus \pz{R_{j-1}}(\pzqi) \pz{p_{j}^{j-1}}$
        
    \State\hspace{0.2in}$ \pz{R_j}(\pzqi) \leftarrow  \pz{R_{j-1}}(\pzqi)  \pz{R_{j}^{j-1}}(\pzqji)$ 
    
    \State\hspace{0.2in}$\pz{\FK_j}(\pzqi) \leftarrow \{ \pz{R_j}(\pzqi) ,  \pz{p_j}(\pzqi) \}$ 
     
    %  \State\hspace{0.4in}{\bf for} $l = 1:j$

    %     \State\hspace{0.6in}$\pzi{R}, \pzi{\nom{p}} \leftarrow \texttt{pzTransMat}(\pzi{q_j})$ 
    
    %     \State\hspace{0.6in}$\pzi{\pj} \leftarrow \pzi{\pj} \oplus \pzi{\Rj} \odot \pzi{p_{l}^{l-1}}$
        
    %     \State\hspace{0.6in}$\pzi{\Rj} \leftarrow \pzi{\Rj} \odot  \pz{R\lssmu}$ 

    % \State\hspace{0.4in}{\bf end for}
    
    % \State\hspace{0.4in}$\pz{\FK_j} \leftarrow \{ \pz{\Rj} ,  \pz{\pj} \}$ 

\State{\bf end for} %\hspace{0.2in}

% \State{\bf end parfor}

\end{algorithmic}
\caption{\small $\{\pzi{\FK_j}\,:\, j \in \Ne,\ i \in \Nt \} = \texttt{PZFK}(\{ \pzi{q_j} \,:\, j \in \Ne,\ i \in \Nt \})$}
\label{alg:compose_fk}
\end{algorithm}

% \State\hspace{0in}{\bf for} $j = 1:\nq$ %// for each joint

%     % \State\hspace{0.2in}$\pz{R_{j}^{j-1}}(\pzqji), \pz{\nom{p\jssmu}} \leftarrow \texttt{pzTransMat}(\pzi{q_j})$ 

% \State\hspace{0in}{\bf end for}

% % \State{\bf end parfor}

% \end{algorithmic}
% \caption{\small $\{\pz{\FK_j}(\pzqi)\,:\, j \in \Nq \} = \texttt{PZFK}(\pzqi)$}
% \label{alg:compose_fk}
% \end{algorithm}

%~~~~~~~~~~~~ Compose FK
\begin{algorithm}[t]
\small
\begin{algorithmic}[1]

% \State{\bf parfor} $i \in \Nt$ %// parallel for each time step

\State{\bf for} $j = 1:\nq+1$ %// for each joint \hspace{0.2in}
    \State\hspace{0.2in}$\pzi{p_j} \leftarrow \pz{\mathbf{0}}$ %// initialize frame location 
        
    \State\hspace{0.2in}$\pzi{\R_j} \leftarrow \pz{I_{3 \times 3}}$ %// initialize frame orientation
    
     \State\hspace{0.2in}{\bf for} $l = 1:j$

        \State\hspace{0.4in}$\pzi{R\lssmu}, \pzi{\nom{p\lssmu}} \leftarrow \texttt{pzTransMat}(\pzi{q_j})$ 
    
        \State\hspace{0.4in}$\pzi{p_j} \leftarrow \pzi{p_j} \oplus \pzi{R_j} \odot \pzi{p_{l}^{l-1}}$
        
        \State\hspace{0.4in}$\pzi{R_j} \leftarrow \pzi{R_j} \odot  \pzi{R\lssmu}$ 

    \State\hspace{0.2in}{\bf end for}
    
    \State\hspace{0.2in}$\pzi{\FO_j} \leftarrow \pzi{p_j} \oplus  \pzi{R_j} \odot \pzi{L_j}$

\State{\bf end for} % \hspace{0.2in}

% \State{\bf end parfor}

\end{algorithmic}
\caption{\small $\{\pzi{\FO_j}\,:\, j \in \Ne,\ i \in \Nt \} = \texttt{PZFO}(\{ \pzi{q_j} \,:\, j \in \Ne,\ i \in \Nt \})$}
\label{alg:compose_fo}
\end{algorithm}
