# Supplementary material for: Serving Time: Real-Time, Safe Motion Planning and Control for Manipulation of Unsecured Objects
Source: arXiv:2309.03111 source file (2023-09-06)
Supplement: Supplementary file 5 [file appendix_4.tex]

\section{Reformulation of Contact Constraints for PZ Overapproximation}
\label{app:constraint_reform}

The contact constraints are formed using $\pz{w^{n_q+1}_{n_q+1}}(\pzqAi, \intparams)$, which is the overapproximation of the contact wrench between the tray and loose object. % \pzi{\cwrenchPZ}
		 
For the separation constraint, the normal component of the contact force is overapproximated by $\pzi{f_{\contact,z}}$, i.e., for each $k\in\pz{K}$ 
\begin{equation}
    f_{\contact,z}(\qA(t;k),\Delta)  \in  \pz{f_{\contact,z}}(\pzqAki,\intparams), \quad \forall t \in \pz{T_i}
\end{equation}
In order to ensure satisfaction of \eqref{eq:optsepcon}, the polynomial zonotope version of the constraint entails choosing $k$ such that
\begin{equation}
    \label{eq:pz_sepcon}
    % - \pzi{\czforcenotPZ} \leq 0, &\quad  \forall i \in \{1,\hdots,\nt\}
    \text{sup}(- \pz{f_{\contact,z}}(\pzqAki,\intparams)) \leq 0, \quad  \forall i \in \{1,\hdots,\nt\}
\end{equation}
Since this constraint is conservatively overapproximative of the actual normal force applied, it is guaranteed that there is a normal force between the loose object and tray when this constraint is satisfied.

The friction constraint, reformulated in Appendix \ref{app:slip_proof}, is addressed next.
Like the normal component of the contact force, the tangential components are overapproximated by elements of $\pzi{\cwrenchPZ}$.
In particular, for each $k \in K$
\begin{equation}
\begin{split}
    f_{\contact,x}(\qT(t;k),\Delta) \in \pz{f_{\contact,x}}(\pzqAki,\intparams)) \quad \forall t \in \pz{T_i} \\
    f_{\contact,y}(\qT(t;k),\Delta)  \in  \pz{f_{\contact,y}}(\pzqAki,\intparams))  \quad \forall t \in \pz{T_i} 
\end{split}
\end{equation}
The polynomial zonotope terms can be substituted into \eqref{eq:linslip}. 

\begin{equation}
    \begin{split}
         \label{eq:linSlipPZ}
         \pz{\slip}(\pzqAi,\intparams) := \pz{f_{\contact,x}}(\pzqAi,\intparams) \pz{f_{\contact,x}}(\pzqAi,\intparams) \\
         \oplus \pz{f_{\contact,y}}(\pzqAi,\intparams)\pz{f_{\contact,y}}(\pzqAi,\intparams) \\
         \ominus \CoefFric^2\pz{f_{\contact,z}}(\pzqAi,\intparams)\pz{f_{\contact,z}}(\pzqAi,\intparams)
    \end{split}
\end{equation}
Then, the polynomial zonotope version of the constraint in \eqref{eq:optslipcon} can be written as
\begin{equation}
    \label{eq:pzslipcon_appendix}
    \sup(\pz{\slip}(\pzqAki,\intparams)) \leq 0
\end{equation}

Note that the coefficient of static friction, $\CoefFric$, could be uncertain, meaning that the actual coefficient exists in an interval $\CoefFric \in [\mu_{s, lower},\mu_{s, upper}]$.
However, it is only necessary to consider the smallest possible value to ensure no slip occurs, so in \eqref{eq:linSlipPZ}, $\CoefFric=\mu_{s, lower}$, since the static coefficient of friction is always a positive number.
By choosing $k$ such that \eqref{eq:pzslipcon_appendix} is satisfied $\forall i \in \{1,\hdots,\nt\}$, it is guaranteed that the object does not translate tangentially to the support surface.

The tipping constraint must also be reformulated to work with polynomial zonotope objects.
The calculation of the tipping constraint, as shown in \eqref{eq:tipConstraint}, requires a square root operation in order to evaluate the $l^2$-norm, which does not currently exist for polynomial zonotopes.
Therefore, we rewrite the constraint as follows:

\begin{equation}
    \lVert \eenorm{} \times \cmoment(\qT(t)) \rVert_2 - \objrad \left| \eenorm{} \cdot \cforce(\qT(t)) \right| \leq 0
\end{equation}
\begin{equation}
    \lVert \eenorm{} \times \cmoment(\qT(t)) \rVert_2 \leq \objrad \left| \eenorm{} \cdot \cforce(\qT(t)) \right|
\end{equation}
\begin{equation}
    \sqrt{(\eenorm{} \times \cmoment(\qT(t)))^2} \leq \objrad \left| \eenorm{} \cdot \cforce(\qT(t)) \right|
\end{equation}
\begin{equation}
    (\eenorm{} \times \cmoment(\qT(t)))^2 \leq \objrad^2 (\eenorm{} \cdot \cforce(\qT(t)))^2
\end{equation}
\begin{equation}
    \label{eq:tipcon_appendix_reform}
    (\eenorm{} \times \cmoment(\qT(t)))^2 - \objrad^2 (\eenorm{} \cdot \cforce(\qT(t)))^2 \leq 0
\end{equation}

% \begin{equation}
%     \left\lVert \frac{\eenorm{} \times \cmoment}{\eenorm{} \cdot \cforce} \right\rVert_2 - \objrad \leq 0
% \end{equation}
% \begin{equation}
%     \label{eq:tipcon}
%     \left\lVert \frac{\eenorm{} \times \cmoment}{\eenorm{} \cdot \cforce}\right\rVert \leq \objrad
% \end{equation}
% where the denominator evaluates to a scalar and the numerator evaluates to a 3x1 vector.
% Since it is chosen that the z-axis of the contact frame is aligned with the normal $\eenorm$ of the supporting surface, the vector $\eenorm{} \times \cmoment$ has a z-axis component that is always zero. 
% Let $[a,b,0]^T$ represent a generic vector resulting from the operation in the numerator which is expressed in the contact frame and let $d$ be a generic value resulting from the operation in the denominator. Then,
% \begin{equation}
%     \left\lVert 
%     \begin{bmatrix}
%         a/d \\
%         b/d \\
%         0
%     \end{bmatrix}
%     \right\rVert \leq \objrad
% \end{equation}
% which can be rewritten as 
% \begin{equation}
%     (a/d)^2 + (b/d)^2 \leq \objrad^2
% \end{equation}
% with the reformulated constraint written as:
% \begin{equation}
%     \label{eq:reform_tipcon}
%     a^2 + b^2 - d^2 \objrad^2 \leq 0
% \end{equation}

Overapproximations of these components are calculated in order to form the polynomial zonotope overapproximation of the tipping constraint.
First, we have that for each $k \in \pz{K}$
\begin{equation}
    \cwrench(\qT(t;k),\Delta) \in \pz{\cwrenchPZ}(\pzqAki,\intparams) \quad \forall t \in \pz{T_i}
\end{equation}
This means that the contact force and moment vector can be overapproximated by the corresponding components of the wrench overapproximation
\begin{equation}
    \begin{split}
        \cmoment(\qT(t;k),\Delta) \in \pz{n_{o}}(\pzqAki,\intparams) \quad \forall t \in \pz{T_i} \\
        \cforce(\qT(t;k),\Delta) \in \pz{f_{o}}(\pzqAki,\intparams) \quad \forall t \in \pz{T_i}
    \end{split}
\end{equation}

The contact force and moment vector overapproximations can be substituted into \eqref{eq:tipcon_appendix_reform}. 
The polynomial zonotope overapproximation of the cross product in \eqref{eq:tipcon_appendix_reform} is
\begin{equation}
    \label{eq:pz_ZMP_numerator}
    \eenorm{} \otimes \pz{n_{o}}(\pzqAi,\intparams) = 
    \begin{bmatrix}
        \pz{a}(\pzqAi,\intparams) \\
        \pz{b}(\pzqAi,\intparams) \\
        0
    \end{bmatrix}
\end{equation}
and the overapproximation of the dot product in \eqref{eq:tipcon_appendix_reform} is
\begin{equation}
    \label{eq:pz_ZMP_denominator}
    \eenorm{} \odot \pz{f_{o}}(\pzqAi,\intparams) = \pz{d}(\pzqAi,\intparams)
\end{equation}
Thus an overapproximation of \eqref{eq:tipConstraint} can be written as
\begin{equation}
    \label{eq:pz_tipcon}
    \begin{split}
        \pz{\tip}(\pzqAi,\intparams) = & \pz{a}(\pzqAi,\intparams) \pz{a}(\pzqAi,\intparams) \\
        & \oplus \pz{b}(\pzqAi,\intparams) \pz{b}(\pzqAi,\intparams) \\
        & \ominus \pz{d}(\pzqAi,\intparams) \pz{d}(\pzqAi,\intparams) \objrad^2
    \end{split}
\end{equation}
Then, the polynomial zonotope version of the constraint can be written as 
\begin{equation}
    \label{eq:APPtipConstraint}
    \text{sup}(\pz{\tip}(\pzqAki,\intparams)) \leq 0
    % \begin{split}
    %     \pz{a}(\pzqAi,\intparams) \pz{a}(\pzqAi,\intparams) & \\
    %     \oplus \pz{b}(\pzqAi,\intparams) \pz{b}(\pzqAi,\intparams) & \\
    %     \ominus \pz{d}(\pzqAi,\intparams) \pz{d}(\pzqAi,\intparams) \objrad^2 & \leq 0
    % \end{split}
\end{equation}
Similar to the coefficient of friction, the radius of the contact area could be uncertain but only the smallest possible value needs to be considered in order to guarantee that no tipping occurs.
Therefore, in \eqref{eq:pz_tipcon}, if $\objrad \in [\objrad_{lower},\objrad_{upper}]$, then $\objrad = \objrad_{lower}$, since the radius must be a positive quantity.
