# Supplementary material for: Serving Time: Real-Time, Safe Motion Planning and Control for Manipulation of Unsecured Objects
Source: arXiv:2309.03111 source file (2023-09-06)
Supplement: Supplementary file 6 [file appendix_6.tex]

\section{Controller Implementation Details}
\label{app:controller_implement}

We use the same controller as presented in \cite[Sec. VII]{michaux2023}, with a different $K_{r}$, $\roblevel$ and $\sigma_m$.
In particular, we let $\roblevel = 2.0 \times 10^{-2}$ which together with the bound on the smallest eigenvalue $\sigma_m$,  yields the uniform bound $
% \begin{equation}
    ||\robr|| \leq \ultbound = \sqrt{\frac{2 \times 2.0 \times 10 ^ {-2}}{8.0386}} \approx 0.0705$.
% \end{equation}
Applying Lem. \ref{lem:tracking_bounds} yields $\pboundj \approx 0.0176 \text{ rad}$ and $\vbound \approx 0.1411 \text{ rad/s}$.
We let $K_{r} = 4I_{7x7}$ where $I_{7x7}$ is a $7x7$ identity matrix.
